# Supplementary material for: Tensor-Network-Based Distributed Quantum Dynamics on Independent Quantum Computers
Source: arXiv:2606.11579 source file (2026-06-10)
Supplement: Supplementary file 1 [file Appendix-B.tex]

\section{Modified phase estimation for energy differences using tensor networks}
\label{appendix-FT}
As noted in the main paper, the phase estimation algorithm provides an approach to compute the eigenstates of a Hamiltonian from time-propagation followed by Fourier transforms. But, in most chemical applications, including vibrational spectroscopy, energy differences are experimentally observed and have chemical meaning, but absolute energies do not have any physical meaning. For example, in molecular spectroscopy, energy differences between eigenvalues are measured and not absolute eigenenergies. Compare this aspect with Eq. (\ref{PEA-Final-main}) which results in spectral intensities at absolute energy values given by $E_e$.  Hence we begin our approach here towards energy differences to arrive at a reduced quantum resource phase estimation using the Fourier transform of the density-density autocorrelation function: 
\begin{comment}
\begin{align}
    \int_{-\infty}^{+\infty} & dt\, %\exp{{\imath \omega t}} 
    e^{{\imath \omega t}} \; {\text{Tr}}[\rho(0)\rho(t)] \nonumber \\ =& 
    \int_{-\infty}^{+\infty} dt\,  
    e^{{\imath \omega t}} \; {\text{Tr}}[\ket{\chi(0)}\bra{\chi(0)}
    %\exp{-\imath H t / \hbar} 
    \ket{\chi(t)}\bra{\chi(t)} %\exp{\imath H t / \hbar}
    ] 
    \nonumber \\ 
    =& 
    \int_{-\infty}^{+\infty} dt\, %\exp{{\imath \omega t}} 
    e^{{\imath \omega t}} \; {\left\vert \bra{\chi(0)}\ket{\chi(t)} \right\vert}^2\nonumber \\ 
    %&= {\left\vert \bra{\chi(0)} \ket{\xi(\omega)} \right\vert}^2
\end{align}
\end{comment}
%Here $\rho(t) = \ket{\chi(t)}\bra{\chi(t)}$ and  $\chi(t)$ is the state of the circuit in Figure \ref{Fig:PEA-ckt1} at ``Stage 2'', Eq. (\ref{Stage2=chi-t}). When the initial wavepacket $\chi(0)$ is written in the eigenbasis $\left\{ E_j; \phi_j \right\}$ with complex coefficients $c_j(0)$, we obtain,
\begin{widetext}
\begin{align}
    \int_{-\infty}^{+\infty} & dt\, %\exp{{\imath \omega t}} 
    e^{{\imath \omega t}} \; {\text{Tr}}[\rho(0)\rho(t)] \nonumber \\ =& \int_{-\infty}^{+\infty} dt\, e^{{\imath \omega t}}
    %\exp{{\imath \omega t}} 
    \; {\text{Tr}}\left[\ket{\chi(0)}\bra{\chi(0)}  \sum_{i,j}c_{i}(0)c_{j}^{*}(0) %\exp(-\frac{i(E_{i}-E_{j})t}{\hbar})
    e^{\imath (E_{i}-E_{j}) t/{\hbar}}
    \ket{\phi_{i}}\bra{\phi_{j}}\right] 
    \nonumber \\ =& \int_{-\infty}^{+\infty} dt\, e^{{\imath \omega t}}
    %\exp{{\imath \omega t}} 
    \; \sum_{i,j} |c_{i}(0)|^2 |c_{j}(0)|^2 %\exp(-\frac{i(E_{i}-E_{j})t}{\hbar})
    e^{\imath (E_{i}-E_{j}) t/{\hbar}} \nonumber \\ 
=& \sum_{i,j}|c_{i}(0)|^{2}|c_{j}(0)|^{2} \; \delta \left(\omega-(E_{i}-E_{j})/\hbar \right),
    \label{Eq:Density-timecorrelation-FT}
\end{align}
\end{widetext}
Here $\rho(t) = \ket{\chi(t)}\bra{\chi(t)}$ and  $\chi(t)$ is the state of the circuit in Figure \ref{Fig:PEA-ckt1} at ``Stage 2'' (Eq. (\ref{Stage2=chi-t}). The initial wavepacket $\chi(0)$ is written in the eigenbasis $\left\{ E_j; \phi_j \right\}$ with complex coefficients $c_j(0)$.
\begin{comment}
\begin{widetext}
%\begin{eqnarray}
\begin{align}
    \int_{-\infty}^{+\infty} dt\, %\exp{{\imath \omega t}} 
    e^{{\imath \omega t}} \; {\text{Tr}}[\rho(0)\rho(t)] &= \int_{-\infty}^{+\infty} dt\, e^{{\imath \omega t}}
    %\exp{{\imath \omega t}} 
    \; {\text{Tr}}\left[\ket{\chi(0)}\bra{\chi(0)}\sum_{i,j}c_{i}(0)c_{j}^{*}(0) %\exp(-\frac{i(E_{i}-E_{j})t}{\hbar})
    e^{\imath (E_{i}-E_{j}) t/{\hbar}}
    \ket{\phi_{i}}\bra{\phi_{j}}\right] \nonumber \\ 
&=\sum_{i,j}|c_{i}(0)|^{2}|c_{j}(0)|^{2} \; \delta \left(\omega-(E_{i}-E_{j})/\hbar \right),
    \label{Eq:Density-timecorrelation-FT}
\end{align}
%\end{eqnarray}
\end{widetext}
\end{comment}
Equation (\ref{Eq:Density-timecorrelation-FT}) now provides eigen-energy differences at spectral peaks as opposed to absolute eigen-energies in the phase estimation algorithm (see \cref{PEA-Final-main,PEA-Final} and also Appendix \ref{PEA-SDO}). 
%Equation (\ref{Eq:Density-timecorrelation-FT}) may also be written as 
%\begin{widetext}
%\end{widetext}
%Fourier representation of the wavepacket time correlation function. 
In the coordinate representation, we may rewrite the \cref{Eq:Density-timecorrelation-FT} using convolution theorem\cite{Numerical-Recipes} to obtain
\begin{comment}
\begin{align}
\int_{-\infty}^{+\infty} dt\, %\exp{{\imath \omega t}} 
    & e^{{\imath \omega t}} \; {\text{Tr}}[\rho(0)\rho(t)] \nonumber \\ &=
    \int dx dx' \int_{-\infty}^{+\infty} dt\, e^{{\imath \omega t}} \; \rho(x,x';0) \rho(x,x';t) \nonumber \\ &=
    \int dx dx' {\left\vert \int_{-\infty}^{+\infty} dt\, e^{{\imath \omega t}} \rho(x,x';t) \right\vert}^2 \nonumber \\ &=
    \int dx {\left\vert \int_{-\infty}^{+\infty} dt\, e^{{\imath \omega t}} \rho(x,x;t) \right\vert}^2 + 
    \nonumber \\ &\phantom{==}
    \int_{x\neq x'} dx dx' {\left\vert \int_{-\infty}^{+\infty} dt\, e^{{\imath \omega t}} \rho(x,x';t) \right\vert}^2
\end{align}
\end{comment}
\begin{widetext}
    \begin{align}
\int_{-\infty}^{+\infty} dt\, %\exp{{\imath \omega t}} 
    & e^{{\imath \omega t}} \; {\text{Tr}}[\rho(0)\rho(t)] \nonumber \\ &=
    \int dx dx' \int_{-\infty}^{+\infty} dt\, e^{{\imath \omega t}} \; \rho(x,x';0) \rho(x,x';t) \nonumber \\ &=
    \int dx dx' {\left\vert \int_{-\infty}^{+\infty} dt\, e^{{\imath \omega t}} \rho(x,x';t) \right\vert}^2 \nonumber \\ &=
    \int dx {\left\vert \int_{-\infty}^{+\infty} dt\, e^{{\imath \omega t}} \rho(x,x;t) \right\vert}^2 + 
    \int_{x\neq x'} dx dx' {\left\vert \int_{-\infty}^{+\infty} dt\, e^{{\imath \omega t}} \rho(x,x';t) \right\vert}^2
\end{align}
\end{widetext}
To perform the Fourier transform classically, we measure the ion-trap system and obtain the grid point ${|x_k⟩ ; |t_j⟩}$ with probabilities $\rho(x,x;t)$, % This yields the state ${|k⟩ ; |t⟩}$, with probability $\rho(x_k, t_j)$ 
the classical Fourier transform of which yields only the diagonal elements of the equation above, that is
\begin{widetext}
\begin{align}  
    {\cal P} (\omega) & = \int dx {\left\vert \int_{-\infty}^{+\infty} dt\,  e^{{\imath \omega t}} \; \rho(x,x; t) \right\vert}^2 \\
    & = \int dx {\left\vert \int_{-\infty}^{+\infty} dt\,  e^{{\imath \omega t}} \;
    %\right. \right. \nonumber \\ & \left. \left. 
    \sum_{i,j}c_{i}(0)c_{j}^{*}(0) %\exp\left(-\frac{i(E_{i}-E_{j})t}{\hbar}\right)
    e^{\imath (E_{i}-E_{j}) t/{\hbar}}
    {\phi_{i}(x)}
    {\phi_{j}(x)} \right\vert}^2 \nonumber \\
    & = \int dx {\left\vert \sum_{i,j} \delta(\omega-(E_{i}-E_{j})) c_{i}(0)c_{j}^{*}(0) {\phi_{i}(x)}
    {\phi_{j}(x)} \right\vert}^2 ,
    \label{Eq:Density-timecorrelation-FT-3} 
\end{align}
\end{widetext}

As can be seen, these diagonal elements also capture the spectral features depicted by Eq. (\ref{Eq:Density-timecorrelation-FT}) (with different peak intensities), but simplifies the experimental implementation. 
In implementing this expression, in this publication, (and in Refs. \cite{IonQ-Anurag}), we further reduce the experimental cost (measured in terms of number of qubits and number entanglement gates) by obtaining the quantity ${\left\vert \chi(x,t) \right\vert}^2$ %through mid-circuit measurements of the ciruit in Figure 1 
using a quantum computer and constructing its Fourier transform classically. 
%\begin{align}
% {\cal I} (\omega; x) & =\int dt \exp{-\imath E t / \hbar} {\left\vert \chi(x,t) \right\vert}^2
% \label{FT-abs}
%\end{align}
Additionally, by measuring Eq. (\ref{Eq:Density-timecorrelation-FT-3}) we are exercising an extremely critical measurement arm that is available to us on a quantum computer. While standard ensemble average based measurements in chemistry may compute the results from Eq. (\ref{Eq:Density-timecorrelation-FT}), a quantum computer has access to  the wavepacket density information (that is the diagonal elements of the wavepacket density, $\rho(x,x;t)$) at every single grid point. We are simply exercising this option available to us to reduce the needed quantum  resources. 

%However, as will be seen there are a variety of initial wavepackets used here, and hence each resultant wavepacket trajectory would independently lead to the quantities in \cref{Eq:Density-timecorrelation-FT-3}. Thus, in the results section, we have first individually computed the quantity in \cref{Eq:Density-timecorrelation-FT-3} to obtain ${\cal I} (\omega; x) \rightarrow {\cal I}_{\chi_0} (\omega; x)$ and then cumulated these to obtain
\begin{comment}
\begin{align}
\sum_{\forall \chi_0} {\cal I}_{\chi_0} (\omega; x) \rightarrow {\cal P} (\omega)
\label{Eq:integ-Density-timecorrelation-FT-4} 
\end{align}
\end{comment}
%Thermal weights could also be introduced at this stage but it is not done in this paper since these would only affect the peak heights and not the frequencies. 

%One may also write ${\left\vert \xi(x,E) \right\vert}^2 $ as the Fourier transform of a time-correlation function,
%\begin{align}
%{\left\vert \xi(x,E) \right\vert}^2 = \int dt dt' \exp{-\imath E (t - t') / \hbar} \chi(x,t) \chi^*(x,t')
%\end{align}
