# Supplementary material for: Tensor-Network-Based Distributed Quantum Dynamics on Independent Quantum Computers
Source: arXiv:2606.11579 source file (2026-06-10)
Supplement: Supplementary file 2 [file Appendix-Logham.tex]

\section{}
\label{appendix-Logham}
\begin{figure*}[tbp]
    \centering
    \input{Figures/Figure-TN-2SVs}
    \caption{A detailed exposition of \cref{Fig:MPS_tEvo_trotter-a} that precisely outlines how the distributed simulations are carried out. The individual one-dimensional potentials are derived from each one-dimensional propagator as shown, yielding a family of effective one-dimensional Hamiltonians for the system. These individual one-dimensional Hamiltonians are then be independently and concurrently simulated on separate ion-trap quantum computers.}
    \label{Fig:MPS_tEvo_trotter-d}
\end{figure*}

We formulate the Hamiltonian governing wavepacket dynamics in the coordinate representation.

In this framework, the kinetic energy operator along each nuclear degree of freedom is constructed independently using the Distributed Approximating Functional (DAF) approach~\cite{DAFprop,discreteDAF,qwaimd-TCAreview}:
\begin{widetext}
\begin{align}
K(x_i,x_i^{\prime}) 
=&\; K\!\left(\left|x_i-x_i^{\prime}\right|\right) \nonumber \\
=&\; \frac{-\hbar^2}{4m\sigma^3\sqrt{2\pi}}
\exp\!\left[-\frac{(x_i - x_i^\prime)^2}{2\sigma^2}\right]
\sum_{n=0}^{M_{\mathrm{DAF}}/2} \left( \frac{-1}{4} \right)^n \frac{1}{n!} 
H_{2n+2}\!\left( \frac{x_i - x_i^\prime}{\sqrt{2}\,\sigma} \right),
\label{DAFderivative}
\end{align}
\end{widetext}
where $\left\{ H_{2n+2}\left( \frac{ x_i - x_i^\prime }{ \sqrt{2} \sigma} \right) \right\}$ denote even-order Hermite polynomials, and the parameters $M_{\mathrm{DAF}}$ and $\sigma$ control the accuracy and efficiency of the approximate kinetic energy operator.

The DAF representation yields a banded Toeplitz structure for the kinetic energy operator, characterized by matrix elements of the form $K_{ij} \equiv K(|i-j|)$. This structure plays a key role in enabling an efficient mapping of the nuclear Hamiltonian to the form of the ion-trap Hamiltonian, as discussed in Ref.~\onlinecite{Debadrita-Mapping-1D-3Qubits}. The dependence of the kinetic energy operator on the separation between grid points $\ket{x_i}$ and $\ket{x_i^\prime}$ ensures that the operator remains localized in the coordinate basis.

With this construction, the full Hamiltonian can be expressed as

\begin{align}
\hat{H}(\vb{\bar{x}},\vb{\bar{x}}^\prime)
= \sum_i K(x_i,x_i^\prime) 
+ \delta(\vb{\bar{x}}-\vb{\bar{x}}^\prime)\,\hat{V}(\vb{\bar{x}}),
\label{Eq:Hamiltonian}
\end{align}
where $\hat{V}(\vb{\bar{x}})$ is the potential energy operator, diagonal in the coordinate representation and obtained from electronic structure calculations. In contrast to the kinetic term, the potential energy is naturally not separable across dimensions, which introduces additional complexity.

A further challenge in quantum dynamics lies in approximating the action of the time-evolution operator on a state $\ket{\Psi}$, namely $e^{-i\hat{H}\Delta t/\hbar}\ket{\Psi}$. In this work, we adopt the Trotter--Suzuki decomposition~\cite{Campbell1897-tj,Baker1901-cj,Trotter,Suzuki1976-us,Nelson-Trotter,qwaimd}, which provides a systematic approximation whose accuracy is controlled by the time step $\Delta t$.

The time evolution operator $e^{-i\hat{H}\Delta t/\hbar}$ is approximated using a first-order Trotter decomposition~\cite{Trotter,Nelson-Trotter}. Applying this factorization to the Hamiltonian in \cref{Eq:Hamiltonian}, the evolution operator can be written as
\begin{align}
e^{-i\hat{H}\Delta t/\hbar}
&= e^{-i\hat{V}(\vb{\bar{x}})\Delta t/\hbar}
\left\{ \prod_i e^{-i\hat{K}(x_i,x_i^\prime)\Delta t/\hbar} \right\}
+ \mathcal{O}(\Delta t^2) \nonumber \\
&= e^{-i\hat{V}(\vb{\bar{x}})\Delta t/\hbar}
\left\{ \prod_i \tensor*{\mathcal{K}}{^{[i]}}(x_i,x_i^\prime) \right\}
+ \mathcal{O}(\Delta t^2),
\label{Eq:first-order-Trotter}
\end{align}
where $\tensor*{\mathcal{K}}{^{[i]}}(x_i,x_i^\prime)$ denotes the kinetic propagator associated with the $i$th coordinate.  
%constructed using the DAF representation introduced in \cref{DAFderivative}.

A key complication arises from the non-separable nature of the potential energy operator in the coordinate representation. To address this, we express the potential propagator as a tensor network. In two dimensions, this takes the form
\begin{align}
e^{-i\hat{V}(\vb{\bar{x}})\Delta t/\hbar}
= \sum_{\beta=1}^{N_s}
\tensor*{\mathcal{V}}{^{[1]}_{\beta}}(x_1)
\tensor*{\mathcal{V}}{^{[2]}_{\beta}}(x_2),
\label{Eq:UV-TN-1}
\end{align}
where the one-dimensional components are obtained via a Schmidt decomposition~\cite{Schmidt_SVD} of the potential propagator.
\begin{comment}
For higher-dimensional systems, this representation generalizes naturally to a matrix product form,
\begin{align}
e^{-i\hat{V}(\vb{\bar{x}})\Delta t/\hbar}
= \sum_{\bar{\beta}}^{\bar{N}_s}
\tensor*{\mathcal{V}}{^{[1]}_{\beta_1}}(x_1)
\qty[\prod_{j=2}^{N-1}
\tensor*{\mathcal{V}}{^{[j]}_{\beta_{j-1}\beta_j}}(x_j)]
\tensor*{\mathcal{V}}{^{[N]}_{\beta_{N-1}}}(x_N),
\label{Eq:UV-TN-N}
\end{align}
with $\bar{\beta} = (\beta_1,\beta_2,\ldots,\beta_{N-1})$. The truncation parameters $N_s$ and $\bar{N}_s$ control the effective entanglement captured in the representation.
\end{comment}
Combining \cref{Eq:first-order-Trotter,Eq:UV-TN-1} with the MPS form of the wavefunction, the time evolution in two dimensions can be written as
\begin{widetext}
\begin{align}
\psi(\bar{\vb{x}};t+\Delta t)
&= \sum_{\alpha,\beta} \int \dd{x'_1}\dd{x'_2}
\;\qty[\tensor*{\mathcal{V}}{^{[1]}_{\beta}}(x_1)
\tensor*{\mathcal{K}}{^{[1]}}(x'_1,x_1)]
\phi^{[1]}_{\alpha}(x'_1) \nonumber \\
&\quad\times
\qty[\tensor*{\mathcal{V}}{^{[2]}_{\beta}}(x_2)
\tensor*{\mathcal{K}}{^{[2]}}(x'_2,x_2)]
\phi^{[2]}_{\alpha}(x'_2) \nonumber \\
&= \sum_{\alpha,\beta}
\phi^{[1]}_{\alpha,\beta}(x_1,t)\,
\phi^{[2]}_{\alpha,\beta}(x_2,t),
\label{Eq:MPS_tEvo_first_order}
\end{align}
\end{widetext}
where the propagated functions $\phi^{[i]}_{\alpha,\beta}$ incorporate both the initial entanglement index $\alpha$ and the additional index $\beta$ introduced by the Trotterized propagator. Together, these define a combined index $\mu=(\alpha,\beta)$, reflecting the growth of entanglement during evolution.

This structure reveals that the time evolution can be interpreted as a collection of parallel one-dimensional propagations, with the number of streams scaling as the $\alpha\times\beta$ times the number of dimensions, as succinctly illustrated in \cref{Fig:MPS_tEvo_trotter-d}.
\begin{comment}
The corresponding generalization to $N$ dimensions follows directly from \cref{Eq:UV-TN-N}, yielding
\begin{widetext}
\begin{align}
\psi(\bar{\vb{x}};t+\Delta t)
&= \sum_{\bar{\alpha},\bar{\beta}}
\int \prod_j \dd{x'_j} \;
\qty[\tensor*{\mathcal{V}}{^{[1]}_{\beta_1}}(x_1)
\tensor*{\mathcal{K}}{^{[1]}}(x'_1,x_1)]
\phi^{[1]}_{\alpha_1}(x'_1) \nonumber \\
&\quad\times
\qty[\prod_{j=2}^{N-1}
\tensor*{\mathcal{V}}{^{[j]}_{\beta_{j-1}\beta_j}}(x_j)
\tensor*{\mathcal{K}}{^{[j]}}(x'_j,x_j)]
\phi^{[j]}_{\alpha_{j-1},\alpha_j}(x'_j) \nonumber \\
&\quad\times
\qty[\tensor*{\mathcal{V}}{^{[N]}_{\beta_{N-1}}}(x_N)
\tensor*{\mathcal{K}}{^{[N]}}(x'_N,x_N)]
\phi^{[N]}_{\alpha_{N-1}}(x'_N) \nonumber \\
&= \sum_{\bar{\alpha},\bar{\beta}}
\phi^{[1]}_{\alpha_1,\beta_1}(x_1,t)
\qty[\prod_{j=2}^{N-1}
\phi^{[j]}_{\alpha_{j-1}\alpha_j,\beta_{j-1}\beta_j}(x_j,t)]
\phi^{[N]}_{\alpha_{N-1},\beta_{N-1}}(x_N,t),
\label{Eq:MPS_tEvo_first_order-ND}
\end{align}
\end{widetext}
which retains the same parallel structure across all dimensions.
\end{comment}
To establish a direct connection between the tensor-network decomposition and effective one-dimensional quantum dynamics, we next analyze the structure of the individual Trotterized propagator blocks appearing in \cref{Eq:MPS_tEvo_first_order}. Each propagator block corresponds to a one-dimensional propagator obtained from the tensor-network decomposition of the potential propagator and acts independently on the associated MPS tensor of the initial wavepacket.

Motivated by the mapping between reduced-dimensional quantum dynamics and ion-trap Ising Hamiltonians discussed in Ref.~\onlinecite{Debadrita-Mapping-1D-3Qubits}, each tensor-network component of the potential propagator is expressed as
\begin{align}
\nonumber
\mathcal{V}^{[j]}_{\beta}(x_j)
&=
{\cal A}^{[j]}_{\beta}(x_j)
\exp{-\imath V^{[j]}_{\beta}(x_j)\Delta t/2\hbar},
\label{Eq:V-A-S}
\end{align}
where
$\left\{V^{[j]}_{\beta}(x_j)\right\}$ 
%and $\left\{V^{[j]}_{\gamma}(x_j)\right\}$
represent effective one-dimensional potentials extracted from the logarithm of the corresponding propagator terms. Specifically,
\begin{align}
\log {\cal A}^{[j]}_{\beta}(x_j)
&=
\Re\qty[\log \mathcal{V}^{[j]}_{\beta}(x_j)],
\label{Eq:log_A}
\\
V^{[j]}_{\beta}(x_j)
&=
-\frac{2\hbar}{\Delta t}
\Im\qty[\log \mathcal{V}^{[j]}_{\beta}(x_j)].
\label{Eq:log_V}
\end{align}

This representation enables the construction of a family of reduced-dimensional Hamiltonians associated with the first-order Trotter decomposition illustrated in \cref{Fig:MPS_tEvo_trotter-d}. The resulting effective Hamiltonians take the form
\begin{align}
H^{[j]}_{\beta}(x_j,x'_j)
=
K^{[j]}(x_j,x'_j)
+
V^{[j]}_{\beta}(x'_j),
\label{Eq:MPS_Ham_first_order}
\end{align}
where the kinetic contribution remains unchanged while the tensor-network decomposition generates effective one-dimensional potential terms.

In this method, the multidimensional propagation reduces to a collection of coupled one-dimensional propagations that can be executed independently on separate quantum hardware platforms. Consequently, the tensor-network representation decomposes the original multidimensional problem into effective one-dimensional subsystems governed by the Hamiltonians in \cref{Eq:MPS_Ham_first_order}.

For the two-dimensional case, the propagated wavefunction can therefore be written as
\begin{widetext}
\begin{align}
\nonumber
\psi(\bar{\vb{x}};t+\Delta t)
&=
\sum_{\alpha,\beta}
\int \dd{x'_1}\dd{x'_2}
\\
&\quad\times
\qty[
{\cal A}^{[1]}_{\beta}(x_1)\exp{-\imath H^{[1]}_{\beta}(x_1,x'_1)\Delta t/\hbar}
]
\phi^{[1]}_{\alpha}(x'_1)
\nonumber
\\
&\quad\times
\qty[
{\cal A}^{[2]}_{\beta}(x_2)\exp{-\imath H^{[2]}_{\beta}(x_2,x'_2)\Delta t/\hbar}
]
\phi^{[2]}_{\alpha}(x'_2)
\nonumber
\\
&=
\sum_{\alpha,\beta}
\phi^{[1]}_{\alpha,\beta}(x_1,t)
\phi^{[2]}_{\alpha,\beta}(x_2,t),
\label{Eq:MPS_tEvo-LogHam3_first}
\end{align}
\end{widetext}
where the effective one-dimensional Hamiltonians satisfy
\begin{widetext}
\begin{align}
\tensor*{\mathcal{U}}{^{[j]}_{}^{}_{\beta}}(x_j,x'_j)
\equiv
\exp{-\imath H^{[j]}_{\beta}(x_j,x'_j)\Delta t/\hbar}
\equiv
\exp{
-\imath
\qty[
K^{[j]}(x_j,x'_j)
+
V^{[j]}_{\beta}(x'_j)
]
\Delta t/\hbar
}.
\label{Eq:Ham1_first}
\end{align}
\end{widetext}
\begin{comment}
The higher-dimensional generalization follows directly from \cref{Eq:MPS_tEvo_first_order-ND}:
\begin{widetext}
\begin{flalign}
\nonumber
\psi(\bar{\vb{x}};t+\Delta t)
&=
\sum_{\bar{\alpha},\bar{\beta}}
\int \prod_j \dd{x'_j}
\\
&\quad\times
\qty[
{\cal A}^{[1]}_{\beta_1}(x_1)\exp{-\imath H^{[1]}_{\beta_1}(x_1,x'_1)\Delta t/\hbar}
]
\phi^{[1]}_{\alpha_1}(x'_1)
\nonumber
\\
&\quad\times
\qty[
\prod_{j=2}^{N-1}
{\cal A}^{[j]}_{\beta_{j-1}\beta_j}(x_j)\exp{-\imath
H^{[j]}_{\beta_{j-1}\beta_j}(x_j,x'_j)
\Delta t/\hbar}
\phi^{[j]}_{\alpha_{j-1},\alpha_j}(x'_j)
]
\nonumber
\\
&\quad\times
\qty[
{\cal A}^{[N]}_{\beta_N}(x_N)\exp{-\imath H^{[N]}_{\beta_{N-1}}(x_N,x'_N)\Delta t/\hbar}
]
\phi^{[N]}_{\alpha_{N-1}}(x'_N)
\nonumber
\\
&=
\sum_{\bar{\alpha},\bar{\beta}}
\phi^{[1]}_{\alpha_1,\beta_1}(x_1,t)
\qty[
\prod_{j=2}^{N-1}
\phi^{[j]}_{\alpha_{j-1}\alpha_j,\beta_{j-1}\beta_j}(x_j,t)
]
\phi^{[N]}_{\alpha_{N-1},\beta_{N-1}}(x_N,t),
\label{Eq:MPS_tEvo-LogHam3_first-ND}
\end{flalign}
\end{widetext}
with
\begin{align}
H^{[j]}_{\beta_{j-1}\beta_j}(x_j,x'_j)
=
K^{[j]}(x_j,x'_j)
+
V^{[j]}_{\beta_{j-1}\beta_j}(x'_j).
\label{Eq:MPS_Ham_first_order-ND}
\end{align}
\end{comment}
The resulting formulation generates a sequence of effective one-dimensional unitary propagations that can be mapped directly onto independent quantum simulators, as illustrated in \cref{Fig:MPS_tEvo_trotter-d}. Each effective Hamiltonian corresponds to a separate quantum evolution problem and may therefore be executed independently and in parallel across multiple quantum devices. The propagated multidimensional wavefunction is subsequently reconstructed through the tensor-network contraction of these one-dimensional propagated components.

The propagators in \cref{Eq:MPS_tEvo-LogHam3_first} take the form of a sum over products of one-dimensional contributions, thereby generating a correlated multidimensional representation of the dynamics. The extent of these correlations is governed by the tensor-network index $\beta$, which encode the entanglement between different nuclear degrees of freedom. 

%As the number of dimensions increases, the generalization proceeds according to \cref{Eq:MPS_tEvo-LogHam3_first-ND} together with the Hamiltonians in \cref{Eq:MPS_Ham_first_order-ND}. 
The complete dynamics is represented through a collection of one-dimensional Hamiltonians, $H^{[j]}_{\beta}(x_j,x'_j),$
\begin{comment}
\begin{align*}
\left\{
H^{[1]}_{\beta_1}(x_1,x'_1),
%H^{[j]}_{\beta_{j-1}\beta_j}(x_j,x'_j),
%H^{[N]}_{\beta_{N-1}}(x_N,x'_N)
\right\},
\end{align*}
\end{comment}
each of which may be simulated independently on separate quantum hardware. Consequently, the total number of parallel quantum propagations is determined is the product of the number of dimensions and the number of significant $\beta$ values which depict the extent of entanglement in the system.
