# Supplementary material for: Tensor-Network-Based Distributed Quantum Dynamics on Independent Quantum Computers
Source: arXiv:2606.11579 source file (2026-06-10)
Supplement: Supplementary file 3 [file appendix.tex]

\section{Phase estimation for wavepacket dynamics}
The phase estimation algorithm has three parts that are described using the three slices in the circuit implementation presented in Figure \ref{Fig:PEA-ckt1}. At the end of Stage 1, the ancilla qubits are present in a complete superposition state and the system state is defined as 
\begin{align}
    \ket{\text {Stage 1}} = \left\{ \frac{1}{\sqrt{2^a}} \sum_{i=0}^{2^a-1} \ket{i} \right\} \otimes \ket{\chi_0}_q,
    \label{Shor-initial}
\end{align}
where $a$ is the number of ancilla qubits and $q$ is the number of system qubits. The state $\chi_0$ represents some parameterization of the initial wavepacket in the system qubit basis. Following this each anilla basis state stores a discrete time-sample of the unitary evolution as given by, for example, 
\begin{align}
    \frac{1}{\sqrt{2^a}} &\left[ \ket{00\cdots00}_a \ket{\chi_0}_q + \ket{00\cdots01}_a U \ket{\chi_0}_q + \right. \nonumber \\ & \left. \ket{00\cdots10}_a U^2  \ket{\chi_0}_q + \cdots \right] = \nonumber \\ \frac{1}{\sqrt{2^a}} &\left[ \ket{00\cdots00}_a \ket{\chi_0}_q + \ket{00\cdots01}_a \ket{\chi_{\Delta t}}_q + \right. \nonumber \\ & \left. \ket{00\cdots10}_a \ket{\chi_{2\Delta t}}_q + \cdots \right]
    \label{Shor-propagated-1}
\end{align}
where we have assumed that 
$U= \exp\left\{-\imath H \Delta t / \hbar\right\}$. In compact form, \cref{Shor-propagated-1} can be written as,
\begin{align}
     \ket{\text {Stage 2}} = \frac{1}{\sqrt{2^a}} \sum_{i=0}^{2^a-1} \ket{i}_a  \left[ U^i \ket{\chi_0}_q \right].
    \label{Eq:Shor-propagated}
\end{align}
The \cref{Eq:Shor-propagated} represents the state at the end of Stage 2 in Figure \ref{Fig:PEA-ckt1}. Thus, each component of the ancilla basis stores a specific time step, that is 
\begin{align}
     \bra{k}_a \ket{\text {Stage 2}} = \frac{1}{\sqrt{2^a}}  \left[ U^k \ket{\chi_0}_q \right] = \frac{1}{\sqrt{2^a}}  \left[ \ket{\chi_{k\Delta t}}_q \right]
    \label{Shor-propagated}
\end{align}
Specifically, for Figure \ref{Fig:PEA-ckt1} the state at the end of $\text {Stage 2}$ may be written as
\begin{align}
     \frac{1}{\sqrt{2^3}} & \left[ \ket{000} \otimes \ket{\chi_0}_q + \ket{001} \otimes \ket{\chi_{\Delta t}}_q + \ket{010} \otimes \ket{\chi_{2\Delta t}}_q +  \right. \nonumber \\ &\left. \ket{011} \otimes \ket{\chi_{3\Delta t}}_q + \ket{100} \otimes \ket{\chi_{4\Delta t}}_q + \ket{101} \otimes \ket{\chi_{5\Delta t}}_q + \right. \nonumber \\ &\left. \ket{110} \otimes \ket{\chi_{6\Delta t}}_q + \ket{111} \otimes \ket{\chi_{7\Delta t}}_q \right]
    \label{Shor-propagated-Figure1}
\end{align}
In this manner, each time step of wavepacket dynamics is stored on a separate ancilla axis. Finally, the QFT step simply Fourier transforms these discrete time-samples to provide the spectral decomposition from wavepacket dynamics to help compute:
\begin{align}
    \int dt \exp \left\{ \imath E \Delta t / \hbar\right\} \exp\left\{-\imath H \Delta t / \hbar\right\} \ket{\chi_0}
\end{align}
The complexity of this algorithm is two-fold: (a) the efficient quantum circuit or quantum simulation implementation of $\left[ U^k \ket{\chi_0}_q \right]$, and (b) implementation of the $Controlled-U$ operations. In this paper we provide a general solution to the first problem.
