# Supplementary material for: Tensor-Network-Based Distributed Quantum Dynamics on Independent Quantum Computers
Source: arXiv:2606.11579 source file (2026-06-10)
Supplement: Supplementary file 4 [file Appendix-D.tex]

\subsection{Tensor networks for representing $U$ further reduces circuit complexity and yields phase estimation on a distributed architecture}
\label{Sec:TN}

There are two key ideas underlying the experimental implementation presented in this work. First, the quantum circuit for phase estimation is partitioned into two stages, as discussed above, with the system state at Stage~2 obtained via measurement. Second, the unitaries required to generate the Stage~2 state are further simplified using tensor network techniques.

To this end, we represent the initial wavefunction $\chi_0$ as a matrix product state (MPS)~\cite{tensor_network}. In this representation, a wavepacket with $N$ nuclear degrees of freedom is expressed as a multi-configurational expansion~\cite{mctdh-meyer,MLMCTDHWang,Burghardt-MLMCTDH,Otto_POTFIT} of $N$ one-dimensional functions:
\begin{align}
\chi_0(\vb{\bar{x}}) = \sum_{\bar{\boldsymbol\alpha}}^{\bar{\boldsymbol\eta}} 
\qty[\prod_{j=1}^{N} \tensor*{\phi}{^{[j]}_{}^{x_j}_{\alpha_{j-1},\alpha_j}}] = \sum_{\bar{\boldsymbol\alpha}}^{\bar{\boldsymbol\eta}} \tensor*{\phi}{^{\bar{x}}_{\bar{\alpha}}} ,
\label{Eq:MPS_WF}
\end{align}
Here, the dependence on the discrete position basis $\vb{\bar{x}} \equiv (x_1, x_2, \ldots, x_N)$ is encoded in tensor elements parameterized by the local coordinates $x_j$. The tensors $\phi^{[j]}$, which are of second or third order tensors, can thus be interpreted as reduced-dimensional functions associated with each coordinate $x_j$. The superscripts in square brackets $[\cdot]$ label the tensor cores and do not represent tensor indices. The terms $\tensor*{\phi}{^{\bar{x}}_{\bar{\alpha}}}$ now refer to the assoicated product state on the equation in the center. 
\begin{figure}[tbp]
    \subfigure[]{\input{Figures/Figures_MPS_prop}
        \label{Fig:MPS_tEvo_trotter-a}}
    \subfigure[]{\input{Figures/Figure-TN-first-trotter}\label{Fig:MPS_tEvo_trotter-b}}
   \caption{Figure \ref{Fig:MPS_tEvo_trotter-a} illustrates the tensor-network representation of the time evolution of a wavepacket. Figure \ref{Fig:MPS_tEvo_trotter-b} shows the corresponding evolution in its Trotterized formulation. In this representation, the initial state is parameterized by entanglement variables $\alpha$, while the Trotterized propagator is characterized by entanglement variables $\beta$. Together, they define the composite index $\mu = \alpha \times \beta$ that labels the evolved state.}
    \label{Fig:MPS_tEvo_trotter}
\end{figure}

\begin{figure}[tbp]
\centering
\input{Figures/Figures_MPS_prop}
\caption{Time evolution of a wavepacket in a tensor-network representation. The initial state is parameterized by entanglement variables $\alpha$, while the time-evolution propagator is characterized by $\beta$. Their combination defines the composite index $\mu = \alpha \times \beta$, which labels the evolved state.}
\label{Fig:MPS_tEvo_trotter-a}
\end{figure}

The summation is performed over the auxiliary indices $\bar{\boldsymbol\alpha} \equiv (\alpha_0, \alpha_1, \ldots, \alpha_N)$, bounded by $\bar{\boldsymbol\eta} \equiv (\eta_0 = 1, \eta_1, \ldots, \eta_{N-1}, \eta_N = 1)$, such that each index satisfies $\alpha_j \in \{1, \ldots, \eta_j\}$. These parameters, commonly referred to as the \emph{bond dimensions} (or equivalently, entanglement dimensions or Schmidt ranks), determine the number of retained singular values at each bipartition of the system in the Schmidt decomposition~\cite{Nicole-TN}.

\begin{figure}[tbp]
\centering
\subfigure[]{%
    \resizebox{0.28\linewidth}{!}{\input{Figures/dim2_beta2}}}
\hfill
\subfigure[]{%
   \resizebox{0.68\linewidth}{!}{\input{Figures/Figure_dim2_beta2_expanded}}}
\caption{(a) Uniformly controlled gate with single control qubit encoding $\beta$. (b) Sequential decomposition of the same uniformly controlled block-diagonal unitary shown in (a).}
\label{fig:2D_2beta_ucg}
\end{figure}

The unitary operator $\hat{U}$ is expressed in the matrix product operator (MPO) form~\cite{MPO,MPOR} as
\begin{align}
\mel{\bar{\vb{x}}'}{\hat{U}}{\bar{\vb{x}}} 
&= \sum_{\bar{\boldsymbol\beta}} 
\left[ \prod_{j=1}^{N} 
\tensor*{\mathcal{U}}{^{[j]}_{}^{x_j x'_j}_{\beta_{j-1},}_{\beta_j}} 
\right],
\label{Eq:propagator-TN}
\end{align}
where the auxiliary indices $\{\beta_j\}$ encode the entanglement structure of the operator across different degrees of freedom. Each tensor $\mathcal{U}^{[j]}$ represents the one-dimensional effective propagtor to propagate the corresponding one-dimensional function $\phi^{[j]}$ in \cref{Eq:MPS_WF}.

Acting on an initial state $\ket{\chi_0}$, written in matrix product state (MPS) form (\cref{Eq:MPS_WF}), the time-evolved wavefunction becomes
\begin{align}
\chi_{\Delta t}(\bar{\vb{x}}) 
&= \sum_{\bar{\boldsymbol\alpha},\bar{\boldsymbol\beta}} 
\left[
\prod_{j=1}^{N} 
\int dx'_j \;
\tensor*{\mathcal{U}}{^{[j]}_{}^{x_j x'_j}_{\beta_{j-1},}_{\beta_j}}
\tensor*{\phi}{^{[j]}_{}^{x'_j}_{\alpha_{j-1},\alpha_j}}
\right]. 
\label{Eq:MPO_MPS}
\end{align}
This expression corresponds to a contraction of the MPO with the MPS, resulting in a new state whose bond structure is governed jointly by $\alpha$ and $\beta$.

For a two-dimensional system, there is a single entanglement index $\beta$, and for a product initial state the expression simplifies to
\begin{align}
\chi_{\Delta t}(\bar{\vb{x}}) 
&= \sum_{\beta} 
\left[
\prod_{j=1}^{2} 
\int dx'_j \;
\tensor*{\mathcal{U}}{^{[j]}{}^{x_j x'_j}_{\beta}}
\tensor*{\phi}{^{[j]}{}^{x'_j}}
\right], 
\label{Eq:MPS_WF-2D-prod-init}
\end{align}
which can be expressed as the action of a family of $\{U\chi\}$ operations. In principle, these operations can be constructed and executed in parallel on a Quantum-HPC architecture. This parallel structure is illustrated in \cref{Fig:MPS_tEvo_trotter-a,Fig:MPS_tEvo_trotter-d}. 

%This form admits a natural interpretation as a sum over independent propagation channels labeled by $\beta$, where each channel corresponds to a distinct product of one-dimensional propagators. Consequently, the evolution can be viewed as a family of operations $\{U_{\beta}\chi\}$, which can, in principle, be executed in parallel on a Quantum-HPC architecture. This parallel structure is illustrated in \cref{Fig:MPS_tEvo_trotter-a,Fig:MPS_tEvo_trotter-d}.

Equivalently, the same operation can be recast as a block-diagonal matrix acting on an enlarged Hilbert space,
\begin{align}
\hat{U} = \bigoplus_{\boldsymbol{\beta}} U_{\boldsymbol{\beta}},
\end{align}
where each block corresponds to a fixed configuration of the entanglement indices and is given by
\begin{align}
U_{\boldsymbol{\beta}} =
\mathcal{U}^{[1]}_{1,\beta_1}
\mathcal{U}^{[2]}_{\beta_1,\beta_2}
\cdots
\mathcal{U}^{[N]}_{\beta_{N-1},1}.
\end{align}
For the case $\beta = 2$, the operator reduces to
\begin{align}
\hat{U} =
\begin{bmatrix}
\mathcal{U}_1^{[1]} \mathcal{U}_1^{[2]} & 0 \\
0 & \mathcal{U}_2^{[1]} \mathcal{U}_2^{[2]}
\end{bmatrix}.
\end{align}
This structure can be implemented using a uniformly controlled gate with a single control qubit, as shown in \cref{fig:2D_2beta_ucg}.

For $\beta = 4$, the operator consists of four blocks, requiring two control qubits to select the corresponding channel. The associated matrix and circuit representation are shown in \cref{fig:2D_4beta_ucg}, where each computational basis state of the control register encodes a specific value of $\beta$.

In general, for an $N$-dimensional system, the resulting operator admits a block-diagonal structure, as illustrated in \cref{fig:general_ucg_matrix}. This structure maps vi  onto a uniformly controlled gate (UCG), where the entanglement indices $\boldsymbol{\beta}$ are encoded in a control register. The number of required control qubits scales as
\begin{align}
m = (N-1)\log_2(\eta_{\max}),
\end{align}
with $\eta_{\max} = \max_j \eta_j$ denoting the maximum bond dimension across all sites.

Within this representation, the full operator can be expressed as
\begin{align}
\hat{U} =
\sum_{\boldsymbol{\beta}}
\ket{\boldsymbol{\beta}}\bra{\boldsymbol{\beta}}
\otimes U_{\boldsymbol{\beta}},
\end{align}
which corresponds precisely to the structure of a uniformly controlled unitary acting on quantum hardware, as depicted in \cref{fig:general_ucg_circuit}. Additionally, each unitary $\left\{ U_{\boldsymbol{\beta}} \right\} $ is a product state unitary and hence for further simplifications in action

This formulation establishes a direct correspondence between tensor-network contractions, the associated block-diagonal operator structure, and their realization as quantum circuits. In particular, the entanglement indices of the tensor network are {\em elevated} to control qubits, while each contraction path through the network defines a conditionally applied unitary evolution on the target system.
