# Supplementary material for: Tensor-Network-Based Distributed Quantum Dynamics on Independent Quantum Computers
Source: arXiv:2606.11579 source file (2026-06-10)
Supplement: Supplementary file 5 [file Appendix-QSD.tex]

\section{Quantum Shannon Decomposition of the individual, distributed tensor cores}
\label{Sec:QSD}
This appendix provides the full decomposition used to implement the operations $\left\{ \tensor*{\mathcal{U}}{^{[j]}_{}^{x_j x'_j}_{\beta_{j-1},}_{\beta_j}} \tensor*{\phi}{^{[j]}_{}^{x_j}_{\alpha_{j-1},\alpha_j}} \right\}$ discussed in \cref{Sec:TN}.

\begin{figure*}[t]
    \centering
    \includegraphics[width=\textwidth]{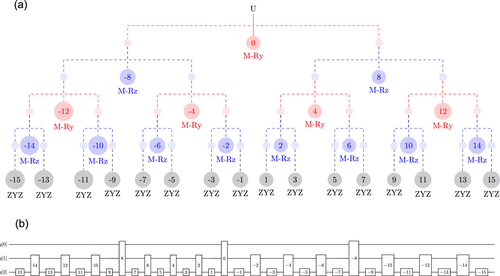}
    \caption{Illustration of the Quantum Shannon Decomposition (QSD) applied to a three-qubit unitary operator \(U\). (a) The unitary is recursively factorized through alternating applications of the cosine--sine decomposition (CSD, shown in red) and the VDW decomposition (shown in blue). The resulting operations include multiplexed rotations \(M\text{-}R_z\) and \(M\text{-}R_y\), corresponding to \(N\)- and \((N-1)\)-qubit multiplexor gates, which can be further expressed as sequences of CNOT gates and single-qubit \(R_z\) or \(R_y\) rotations. The final stage of the decomposition (gray) reduces the remaining operators to single-qubit gates. (b) Quantum circuit representation obtained from the decomposition shown in panel (a). Single-qubit operations acting on \(q[2]\) are expressed using the standard ZYZ Euler-angle decomposition, while the multiqubit components correspond to multicontrolled \(R_y\) and \(R_z\) rotations.}
    \label{Fig:qsd-tree}
\end{figure*}

In this section, we employ the Quantum Shannon Decomposition (QSD) to decompose the unitary propagators arising in quantum dynamical simulations into explicit quantum circuits. The general methodology of QSD has been described in detail in Ref. \cite{Debadrita-water}. Therefore, we summarize here only the key concepts necessary for completeness and for understanding the implementation used in the present study.

The QSD provides a systematic framework for decomposing an arbitrary unitary operator \(U \in U(2^n)\), acting on an n-qubit Hilbert space, into a sequence of elementary quantum gates drawn from a universal gate set. We adopt the universal gate set 
\(\{R_y(\theta), R_z(\theta), \mathrm{CNOT}\}\), where \(R_y(\theta)\) and \(R_z(\theta)\) represent single-qubit rotations about the y- and z-axes of the Bloch sphere, respectively, and \(\mathrm{CNOT}\) is a two-qubit entangling gate. Because this gate set is universal, any unitary transformation can be expressed as a finite sequence of these operations, allowing the resulting circuits to be executed directly on quantum hardware.

The overall structure of the decomposition is illustrated in the tree diagram shown in \cref{Fig:qsd-tree}. The QSD algorithm proceeds through a recursive sequence of matrix factorizations that combine two well-established techniques: the cosine--sine decomposition (CSD)\cite{Golub,sutton2009csd,paige1994historyCSD} and the eigenvalue-based factorization of block-diagonal unitaries, commonly referred to as the VDW decomposition\cite{mottonen12006decompositions}. In \cref{Fig:qsd-tree}, the CSD steps are indicated in red, while the VDW steps are highlighted in blue. Beginning with a unitary matrix \(U\) of dimension \(2^n \times 2^n\), the CSD factorizes the matrix into the form
\begin{equation}
U =
\begin{pmatrix}
L_0 & 0 \\
0 & L_1
\end{pmatrix}
\begin{pmatrix}
\cos \Theta & -\sin \Theta \\
\sin \Theta & \cos \Theta
\end{pmatrix}
\begin{pmatrix}
R_0 & 0 \\
0 & R_1
\end{pmatrix},
\end{equation}
where \(L_0, L_1, R_0,\) and \(R_1\) are unitary matrices of size 
\(2^{n-1}\times 2^{n-1}\), and \(\Theta\) is a diagonal matrix whose entries define rotation angles.

The central cosine--sine block corresponds to a multicontrolled rotation about the \(y\)-axis acting on a single target qubit, commonly denoted as a \(C^{n-1}R_y\) gate. In this construction, the \(n-1\) control qubits select the rotation angle applied to the target qubit according to their computational basis configuration. Each basis state therefore induces a different rotation \(R_y(\alpha_i)\). These multicontrolled operations can be decomposed further into elementary gates using a Gray-code construction\cite{mottonen2004quantum}, resulting in \(2^{n-1}\) CNOT gates and an equal number of single-qubit \(R_y(\theta_i)\) rotations. Although such operations capture the expressive power of quantum circuits, they can be costly in the current NISQ regime because of the large number of entangling gates required.

The remaining block-diagonal matrices produced by the CSD,
\(
\mathrm{diag}(L_0,L_1)
\)
and
\(
\mathrm{diag}(R_0,R_1),
\)
represent another important class of multiqubit operations known as quantum multiplexors. These correspond to conditional transformations in which a single control qubit determines which of two \((n-1)\)-qubit unitary operations is applied to the remaining qubits. This structure differs from that of the CS block: whereas the CS matrix involves multiple control qubits acting on a single target qubit, the multiplexor involves a single control qubit acting on multiple target qubits.

To continue the recursive reduction, the block-diagonal unitaries are further factorized using the VDW scheme. In this approach,
\begin{equation}
\begin{pmatrix}
L_0 & 0 \\
0 & L_1
\end{pmatrix}
=
\begin{pmatrix}
V & 0 \\
0 & V
\end{pmatrix}
\begin{pmatrix}
D & 0 \\
0 & D^\dagger
\end{pmatrix}
\begin{pmatrix}
W & 0 \\
0 & W
\end{pmatrix},
\end{equation}
with an analogous expression for the corresponding right unitary blocks. Here \(V\) and \(W\) are unitary matrices acting on an \((n-1)\)-qubit Hilbert space, while \(D\) is a diagonal unitary matrix. In the circuit representation, the operators \(V\) and \(W\) correspond to lower-dimensional multiqubit gates, thereby effectively reducing the problem size by one qubit. This recursive dimensional reduction is the key mechanism that allows QSD to systematically break down large unitary transformations.

The diagonal matrix \(D\) gives rise to a multicontrolled \(R_z\) rotation, analogous to the multicontrolled \(R_y\) operation originating from the CS block. Using the same Gray-code procedure, this operation can be expressed as a sequence of \(2^{n-1}\) CNOT gates interleaved with \(2^{n-1}\) single-qubit \(R_z(\theta_i)\) rotations. Consequently, both the CS and VDW stages ultimately reduce the original unitary transformation to combinations of controlled rotations together with smaller-dimensional unitary matrices.

\begin{figure}[hbtp]
\begin{center}
\begin{quantikz}[row sep=0.2cm,column sep=0.3cm]
& & \gate[3]{MR_z} & & \gate[3]{MR_y} & & \gate[3]{MR_z} & & \\
& \gate[2]{A_1} & & \gate[2]{B_1} & & \gate[2]{A_2} & & \gate[2]{B_2} & \\
& & & & & & & & \\
\end{quantikz}
\end{center}
\caption{
Three-qubit QSD decomposition grouped into alternating two-qubit and multicontrolled three-qubit subroutines. 
}
\label{fig:qsd7sub}
\end{figure}

By alternating between the CSD and VDW decompositions, the size of the unitary matrices is progressively reduced. After \(n-1\) recursive steps, the remaining operators act on a single qubit. These final single-qubit unitaries are decomposed using the standard ZYZ Euler-angle representation, yielding sequences of \(R_z\) and \(R_y\) rotations.

The resulting circuit obtained from the QSD therefore consists of multicontrolled rotations about the \(y\)- and \(z\)-axes, multiplexor operations, and single-qubit gates. Each of these elements can be systematically expressed in terms of the universal gate set \(\{R_y(\theta), R_z(\theta), \mathrm{CNOT}\}\). In this way, the QSD provides a constructive procedure for converting an arbitrary unitary operator into an explicit quantum circuit suitable for implementation on quantum computing hardware.

The QSD shown in Fig.~\ref{Fig:qsd-tree} requires 24 fully-entangling two-qubit gates to implement an arbitrary three-qubit unitary. For quantum hardware platforms that admit partial-angle entangling gates, such as trapped ions, the circuit depth and complexity may be further reduced. We begin by writing the three-qubit QSD in terms of 7 subroutines, as shown in Fig.~\ref{fig:qsd7sub}.

\begin{figure*}[t]
\begin{center}
\begin{adjustbox}{width=\textwidth}
\begin{quantikz}[row sep=0.2cm,column sep=0.3cm]
& \gate{Z(\theta_1)} & \gate{Y(\theta_3)} & \gate{Z(\theta_5)} & & & \gate[2]{XX(\theta_7)} & \gate{X(\theta_{8})} & & \gate{Y(\frac{\pi}{2})} & \gate[2]{XX(\theta_9)} & \gate{X(\theta_{10})} & \gate{Y(-\frac{\pi}{2})} & \gate{Z(-\frac{\pi}{2})} & \gate[2]{XX(\theta_{11})} & \gate{X(\theta_{12})} & & \gate{Z(\frac{\pi}{2})} & \gate{Z(\theta_{13})} & \gate{Y(\theta_{15})} & \gate{Z(\theta_{17})} &\\
& \gate{Z(\theta_2)} & \gate{Y(\theta_4)} & \gate{Z(\theta_6)} & \gate{Z(-\frac{\pi}{2})} & & & \gate{X(\theta_{8})} & \gate{Z(\frac{\pi}{2})} & \gate{Y(\frac{\pi}{2})} & & \gate{X(\theta_{10})} & \gate{Y(-\frac{\pi}{2})} & & & \gate{X(\theta_{12})} & & & \gate{Z(\theta_{14})} & \gate{Y(\theta_{16})} & \gate{Z(\theta_{18})} &\\
\end{quantikz}
\end{adjustbox}

\vspace{30pt}

\begin{adjustbox}{width=\textwidth}
\begin{quantikz}[row sep=0.2cm,column sep=0.3cm]
& \gate{Z(\theta_1)} & \gate{Y(\theta_3)} & \gate{Z(\theta_5)} & \gate{Z(-\frac{\pi}{2})} & \gate[2]{XX(\theta_7)} & \gate{X(\theta_{8})} & \gate{Z(\frac{\pi}{2})} & \gate{Y(\frac{\pi}{2})} & \gate[2]{XX(\theta_9)} & \gate{X(\theta_{10})} & \gate{Y(-\frac{\pi}{2})} & & \gate[2]{XX(\theta_{11})} & \gate{X(\theta_{12})} & & \gate{Z(\theta_{13})} & \gate{Y(\theta_{15})} & \gate{Z(\theta_{17})} &\\
& \gate{Z(\theta_2)} & \gate{Y(\theta_4)} & \gate{Z(\theta_6)} & & & \gate{X(\theta_{8})} & & \gate{Y(\frac{\pi}{2})} & & \gate{X(\theta_{10})} & \gate{Y(-\frac{\pi}{2})} & \gate{Z(-\frac{\pi}{2})} & & \gate{X(\theta_{12})} & \gate{Z(\frac{\pi}{2})} & \gate{Z(\theta_{14})} & \gate{Y(\theta_{16})} & \gate{Z(\theta_{18})} &\\
\end{quantikz}
\end{adjustbox}

\end{center}
\caption{
Full gate sequence for subroutines $A_{1,2}$ (top) and $B_{1,2}$ (bottom) used in the partial-angle QSD decomposition. Each circuit has 18 adjustable angles $\theta_i$ which are used to specify the desired two-qubit unitary.
}
\label{fig:qsd2qubit}
\end{figure*}

In Fig.~\ref{fig:qsd7sub}, the four subroutines $A_{1,2}$ and $B_{1,2}$ operate only on two qubits and may be fully decomposed using the KAK method. This yields a minimal quantum circuit with 15 single-qubit gates and 3 fully entangling two-qubit operations. In our implementation, the full two-qubit entanglement gates are replaced by partial-angle $XX(\theta)$ gates, with the surrounding single-qubit gates adjusted accordingly. The resulting sequences for these two-qubit unitary subroutines is shown in Fig.~\ref{fig:qsd2qubit}.

\begin{figure*}[t]
\begin{center}
\begin{adjustbox}{width=\textwidth}
\begin{quantikz}[row sep=0.2cm,column sep=0.3cm]
& \gate{Z(\theta_1)} & \gate{Y(\frac{\pi}{2})} & \gate[2]{XX_{12}(\theta_2)} & \gate{X(\theta_{3})} & \gate{Y(-\frac{\pi}{2})} & \gate[3]{XX_{13}(\frac{\pi}{2})} & \gate{X(-\frac{\pi}{2})} & \gate{Y(\frac{\pi}{2})} & \gate[2]{XX_{12}(\theta_4)} & \gate{X(\theta_{5})} & \gate{Y(-\frac{\pi}{2})} & \gate{Z(\theta_6)} & \gate[3]{XX_{13}(\frac{\pi}{2})} & \gate{X(-\frac{\pi}{2})} &\\
& & \gate{Y(\frac{\pi}{2})} & & \gate{X(\theta_{3})} & & & & & & \gate{X(\theta_{5})} & \gate{Y(-\frac{\pi}{2})} & & & &\\
& & \gate{Y(\frac{\pi}{2})} & & & & & \gate{X(\pi)} & & & & & & & \gate{Y(-\frac{\pi}{2})} &\\
\end{quantikz}
\end{adjustbox}

\vspace{30pt}

\begin{adjustbox}{width=\textwidth}
\begin{quantikz}[row sep=0.2cm,column sep=0.3cm]
& \gate{Y(\theta_1)} & \gate{Z(-\frac{\pi}{2})} & \gate[2]{XX_{12}(\theta_2)} & \gate{X(\theta_{3})} & \gate{Z(\frac{\pi}{2})} & \gate[3]{XX_{13}(\frac{\pi}{2})} & \gate{X(-\frac{\pi}{2})} & \gate{Z(-\frac{\pi}{2})} & \gate[2]{XX_{12}(\theta_4)} & \gate{X(\theta_{5})} & \gate{Z(\frac{\pi}{2})} & \gate{Y(\theta_6)} & \gate[3]{XX_{13}(\frac{\pi}{2})} & \gate{X(-\frac{\pi}{2})} &\\
& & \gate{Y(\frac{\pi}{2})} & & \gate{X(\theta_{3})} & & & & & & \gate{X(\theta_{5})} & \gate{Y(-\frac{\pi}{2})} & & & &\\
& & \gate{Y(\frac{\pi}{2})} & & & & & \gate{X(\pi)} & & & & & & & \gate{Y(-\frac{\pi}{2})} &\\
\end{quantikz}
\end{adjustbox}

\end{center}
\caption{
Gate decomposition for multicontrolled three-qubit subroutines $MR_z$ (top) and $MR_y$ (bottom). Each circuit contains 6 adjustable angles $\theta_i$ used to specify the target multicontrolled unitary.
}
\label{fig:qsd3qubit}
\end{figure*}

The full QSD additionally requires three multi-controlled operations acting on all three qubits. In Fig.~\ref{fig:qsd7sub}, subroutines $MR_z$ and $MR_y$ indicate $R_z$ and $R_y$ rotations (respectively), with rotation angles controlled by the four possible states of the top two qubits. In Fig.~\ref{fig:qsd3qubit}, we provide the full decomposition of these subroutines using partial-angle entangling gates. Compared to a typical multicontrolled gate on three qubits, which requires four fully-entangling operations, our decomposition executes the same unitary using two fully-entangling and two partially-entangling operations. In total, six adjustable angles are used to specify the desired $MR_z$ and $MR_y$ subroutines.
